# Supplementary material for: Computation of marginal eigenvalue distributions in the Laguerre and Jacobi $\beta$ ensembles
Source: arXiv:2402.16069 ancillary file (2024-02-25)
Supplement: Supplementary file 1 [file Mathematica_Codes_Description.pdf]

# Computation of marginal eigenvalue distributions in the Laguerre and Jacobi $\beta$ ensembles

Peter J. Forrester[1] and Santosh Kumar[2]

[1]School of Mathematics and Statistics, The University of Melbourne, Victoria 3010, Australia. Email: pjforr@unimelb.edu.au;
[2] Department of Physics, Shiv Nadar Institution of Eminence, Gautam Buddha Nagar, Uttar Pradesh - 201314, India. Email: skumar.physics@gmail.com

## Supplementary Material: Mathematica Codes Description

**Laguerre-A**
This code computes the probability density function (PDF) and cumulative distribution function (CDF) of all ordered eigenvalues for the Laguerre ensemble, Eq. (1.1), with weight function $x^{\lambda_1}e^{-\beta x/2}$, where $\lambda_1$ is a non-negative integer and $\beta$ is a positive integer.

**Laguerre-B**
This code computes the probability density function PDF and CDF of all ordered eigenvalues for the Laguerre ensemble, Eq. (1.1), with weight function $x^{\lambda_1}e^{-\beta x/2}$, where $\lambda_1 + 1/2$ is a non-negative integer and $\beta = 1$.

**Laguerre-C**
This code computes the PDF and CDF of all ordered eigenvalues for the Laguerre ensemble, Eq. (1.1), with weight function $x^{\lambda_1}e^{-\beta x/2}$, where $\lambda_1 + 1/2$ is a non-negative integer and $\beta$ is a positive odd-integer.

**Laguerre-FixedTrace-A**
This code computes the PDF and CDF of all ordered eigenvalues for the fixed (unit) trace Laguerre ensemble, Eq. (3.1), with weight function $x^{\lambda_1}$, where $\lambda_1$ is a non-negative integer. Also, $\beta$ is a positive integer. This code corresponds to the unconstrained trace case of Laguerre-A above.

**Laguerre-FixedTrace-B**
This code computes the PDF and CDF of all ordered eigenvalues for the fixed (unit) trace Laguerre ensemble, Eq. (3.1), with weight function $x^{\lambda_1}$, where $\lambda_1 + 1/2$ is a non-negative integer. The $\beta$ value is 1. This code corresponds to the unconstrained trace case of Laguerre-B above.

**Laguerre-FixedTrace-C**
This code computes the PDF and CDF of all ordered eigenvalues for the fixed (unit) trace Laguerre ensemble, Eq. (3.1), with weight function $x^{\lambda_1}$, where $\lambda_1 + 1/2$ is a non-negative integer. The parameter $\beta$ takes positive odd-integer values. This code corresponds to the unconstrained trace case of Laguerre-C above.

**Jacobi-A**
This code computes the PDF and CDF of all ordered eigenvalues for the Jacobi ensemble, Eq. (1.2), with weight function $x^{\lambda_1}(1-x)^{\lambda_2}$, where $\lambda_1 > -1$, $\lambda_2$ is a non-negative integer, and $\beta$ is a positive integer.

**Jacobi-B**
This code computes the PDF and CDF of all ordered eigenvalues for the Jacobi ensemble, Eq. (1.2), with weight function $x^{\lambda_1}(1-x)^{\lambda_2}$, where $\lambda_1$ is a non-negative integer, $\lambda_2 > -1$, and $\beta$ is a positive integer.

**CondDist**
This code computes the PDF of Landauer conductance for a two terminal chaotic mesoscopic cavity supporting $N_1$ and $N_2$ number of channels for $\beta = 1$ case, when $|N_1 - N_2|$ is an even integer.

**GeneratingFunctionZeros**
This code computes the zeros of the generating function $\Xi_N(z;x)$ of the gap probabilities associated with the eigenvalues. This has to be used along with one of the above mentioned codes which compute the explicit CDF expressions.
